# Supplementary material for: A Step Toward Deep Online Aggregation (Extended Version)
Source: arXiv:2303.04103 source file (2023-03-07)
Supplement: Supplementary file 1 [file 10_supplement.tex]

\section{Experiment Setup Details}

\subsection{WanderJoin}
Add modified queries here.

\subsection{Presto}
\begin{itemize}
    \item Note down versions of each program.
    \item Created an HDFS storage. With Parquet format.
    \item Created a MySQL backed Hive Metastore.
    \item Created a TPC-H Schema with Parquet File Inputs.
    \item Loaded the data from available parquet files into the pre-defined tables. The files were already partitioned (512M. Same as \system's partitions).
    \item Ran the presto server on a single node with the following memory config: JVM Max: 48GB, Max-Memory Per Node: 30GB. Lower than JVM memory because of Heap Headroom requirement.
\end{itemize}
